# Supplementary material for: High-level ab initio quartic force fields and spectroscopic characterization of C$_{2}$N$^{-}$
Source: arXiv:2111.07150 source file (2021-11-13)
Supplement: Supplementary file 1 [file sup_mat.pdf]

# High-level ab initio quartic force fields and spectroscopic characterization of $C_2N^-$

C. M. R. Rocha[1] and H. Linnartz

*Laboratory for Astrophysics, Leiden Observatory, Leiden University, P.O. Box 9513, NL-2300 RA Leiden, The Netherlands.*

# Electronic Supplementary Information

[1]Corresponding author. E-mail address: romerorocha@strw.leidenuniv.nl

# Summary

**1) SPECTRO input for** $\ell$**-**$CCN^-(^3\Sigma^-)$

**2) SPECTRO input for** $c$**-**$CNC^-(^1A_1)$

**3) Parameters employed in the rovibrational DVR3D calculations**

**4) Benchmark calculations: general results**

**5) Convergence of equilibrium geometries with respect to energy increments**

**6) Nuclear spin-rotation hyperfine tensors for** $\ell$**-**$CCN^-(^3\Sigma^-)$ **and** $c$**-**$CNC^-(^1A_1)$

**7) Simulated rotational spectra of** $\ell$**-**$CCN^-(^3\Sigma^-)$ **and** $c$**-**$CNC^-(^1A_1)$ **at** $T = 100\,\mathrm{K}$

**8) PGOPHER file for** $\ell$**-**$CCN^-(^3\Sigma^-)$

**9) PGOPHER file for** $c$**-**$CNC^-(^1A_1)$

**10) Simulated rotational spectra of** $\ell$**-**$CCO(^3\Sigma^-)$ **at** $T = 10\,\mathrm{K}$

```
# SPECTRO ###########################################
    02    0    2    0    1    0    0    4    0    0   00    2    2    0    0
     0    1    0    0    0    1    0    0    0    0    0    0    0    0    0
# GEOM ########################################
   3   1
 7.00         0.000000000         0.000000000        -2.27467474151324
 6.00         0.000000000         0.000000000         0.00000000000000
 6.00         0.000000000         0.000000000         2.56886840390461
# LABELS ############################################
2    3
3    2
# FERMI1 ###########################################
1
2    3
# CURVIL ###########################################
     1    2
     3    2
     2    1    3
# DEGMODE #####
     2    1    0
     1    3
     2
     4
# F2INT #######
    10
     1    1                  12.3643019994
     2    1                   2.0839285054
     3    1                   0.0000000000
     4    1                   0.0000000000
     2    2                   5.4913699270
     3    2                   0.0000000000
     4    2                   0.0000000000
     3    3                   0.4141452281
     4    3                   0.0000000000
     4    4                   0.4141452281
# F3INT #######
    20
     1    1    1            -94.3113195116
     2    1    1              2.4760757084
     3    1    1              0.0000000000
     4    1    1              0.0000000000
     2    2    1             -6.9086955905
     3    2    1              0.0000000000
     4    2    1              0.0000000000
     3    3    1             -0.8749187022
     4    3    1              0.0000000000
     4    4    1             -0.8749187022
     2    2    2            -38.6440217450
     3    2    2              0.0000000000
     4    2    2              0.0000000000
     3    3    2             -0.4844215654
     4    3    2              0.0000000000
     4    4    2             -0.4844215654
     3    3    3              0.0000000000
     4    3    3              0.0000000000
     4    4    3              0.0000000000
     4    4    4              0.0000000000
# F4INT #######
    35
     1    1    1    1       497.6683088840
```

| | | | | |
|---|---|---|---|---|
| 2 | 1 | 1 | 1 | 21.1112698245 |
| 3 | 1 | 1 | 1 | 0.0000000000 |
| 4 | 1 | 1 | 1 | 0.0000000000 |
| 2 | 2 | 1 | 1 | −17.7900240513 |
| 3 | 2 | 1 | 1 | 0.0000000000 |
| 4 | 2 | 1 | 1 | 0.0000000000 |
| 3 | 3 | 1 | 1 | −0.3022059814 |
| 4 | 3 | 1 | 1 | 0.0000000000 |
| 4 | 4 | 1 | 1 | −0.3022059814 |
| 2 | 2 | 2 | 1 | 16.3592106505 |
| 3 | 2 | 2 | 1 | 0.0000000000 |
| 4 | 2 | 2 | 1 | 0.0000000000 |
| 3 | 3 | 2 | 1 | 2.4281390368 |
| 4 | 3 | 2 | 1 | 0.0000000000 |
| 4 | 4 | 2 | 1 | 2.4281390368 |
| 3 | 3 | 3 | 1 | 0.0000000000 |
| 4 | 3 | 3 | 1 | 0.0000000000 |
| 4 | 4 | 3 | 1 | 0.0000000000 |
| 4 | 4 | 4 | 1 | 0.0000000000 |
| 2 | 2 | 2 | 2 | 207.8714397514 |
| 3 | 2 | 2 | 2 | 0.0000000000 |
| 4 | 2 | 2 | 2 | 0.0000000000 |
| 3 | 3 | 2 | 2 | −0.7467327173 |
| 4 | 3 | 2 | 2 | 0.0000000000 |
| 4 | 4 | 2 | 2 | −0.7467327173 |
| 3 | 3 | 3 | 2 | 0.0000000000 |
| 4 | 3 | 3 | 2 | 0.0000000000 |
| 4 | 4 | 3 | 2 | 0.0000000000 |
| 4 | 4 | 4 | 2 | 0.0000000000 |
| 3 | 3 | 3 | 3 | 2.1642897777 |
| 4 | 3 | 3 | 3 | 0.0000000000 |
| 4 | 4 | 3 | 3 | 1.2736235634 |
| 4 | 4 | 4 | 3 | 0.0000000000 |
| 4 | 4 | 4 | 4 | 2.1642897777 |

```
# SPECTRO ##############################################
   02     0     2     1     0     0     0     4     1     0    00     2     2     0     0
    1     0     0     0     0     1     0     0     0     0     0     1     0     0     0
# GEOM ##########################################
   3    1
 7.00          0.000000000          0.00000000000000       0.00000000000000
 6.00          0.000000000          1.37268525875691      -2.16527365386260
 6.00          0.000000000         -1.37268525875691      -2.16527365386260
# LABELS #############################################
3     2
2     3
# CORIOL #############################################
1
0
3     2     0     0     1
1     1
# DARLING ##############################################
1
3     2

# CURVIL #############################################
    1     2
    1     3
    1     2     3
# SYMCRD #############################################
1     2     0     0
2     1     2
0.0   1     1
2     1     0     0
1     3
0.0   1
3     2     0     0
2     1     2
0.0   1    -1
# F2INT #######
    6
    1     1                      8.6018373116
    2     1                      3.7014874870
    3     1                      0.0000000000
    2     2                      6.0946522642
    3     2                      0.0000000000
    3     3                      5.4158489038
# F3INT #######
   10
    1     1     1              -37.2384504948
    2     1     1              -11.6436894944
    3     1     1                0.0000000000
    2     2     1              -23.3909471040
    3     2     1                0.0000000000
    3     3     1              -26.7039947528
    2     2     2              -46.5351430907
    3     2     2                0.0000000000
    3     3     2               -2.0260995372
    3     3     3                0.0000000000
# F4INT #######
   15
    1     1     1     1        133.9948601352
    2     1     1     1         29.2795021731
    3     1     1     1          0.0000000000
    2     2     1     1         54.4000520240
```

| | | | | |
|---|---|---|---|---|
| 3 | 2 | 1 | 1 | 0.0000000000 |
| 3 | 3 | 1 | 1 | 103.1417808735 |
| 2 | 2 | 2 | 1 | 119.5040774409 |
| 3 | 2 | 2 | 1 | 0.0000000000 |
| 3 | 3 | 2 | 1 | −18.9583683304 |
| 3 | 3 | 3 | 1 | 0.0000000000 |
| 2 | 2 | 2 | 2 | 316.2356747980 |
| 3 | 2 | 2 | 2 | 0.0000000000 |
| 3 | 3 | 2 | 2 | −41.5885347650 |
| 3 | 3 | 3 | 2 | 0.0000000000 |
| 3 | 3 | 3 | 3 | 74.0690985068 |

Table S1: Parameters employed in the rovibrational DVR3D calculations [a].

| Parameter | $\ell$-CCN$^-$($^3\Sigma^-$) | $c$-CNC$^-$($^1A_1$) |
|---|---|---|
| NPNT1[b] | 40 | 40 |
| NPNT2[b] | 56 | 56 |
| NALF[c] | 80 | 80 |
| $r_{\mathrm{e},1}/\mathrm{a}_0$[d] | 2.5689 | 2.7454 |
| $D_{\mathrm{e},1}/\mathrm{E_h}$ | 0.1145 | 0.2099 |
| $w_{\mathrm{e},1}/\mathrm{E_h}$ | 0.0057 | 0.0056 |
| $r_{\mathrm{e},2}/\mathrm{a}_0$ | 3.5591 | 2.1653 |
| $D_{\mathrm{e},2}/\mathrm{E_h}$ | 0.2179 | 0.3375 |
| $w_{\mathrm{e},2}/\mathrm{E_h}$ | 0.0085 | 0.0080 |

[a] Jacobi coordinates have been employed throughout. Radial and angular bases are represented by Morse oscillator-like functions and (associated) Legendre polynomials, respectively. The same parameters are utilized for the rare isotopologues.
[b] Number of DVR points in $r_i (i = 1, 2)$ from Gauss-(associated) Laguerre quadrature.
[c] Number of DVR points in $\theta$ from Gauss-(associated) Legendre quadrature.
[d] $r_{\mathrm{e},i}$, $D_{\mathrm{e},i}$ and $w_{\mathrm{e},i}$ are the equilibrium separation, fundamental frequency and dissociation energy of the relevant coordinate $r_i (i=1, 2)$, respectively.

**go to summary**

Table S2: Internal coordinate force constants for $c$-$H_2O(^1A_1)$, $\ell$-HCN($^1\Sigma_g^+$), and $\ell$-CCO($^3\Sigma^-$) model systems taken from our final composite QFFs [Eqs. (2) and (7) of the manuscript]. Units are mdyn Å$^{-n}$rad$^{-m}$ appropriate for an energy unit of mdyn Å($\equiv$ aJ). See Eqs. (3)-(6) in the original paper for the coordinates.

| | $c$-$H_2O(^1A_1)$[a] | $\ell$-HCN($^1\Sigma_g^+$)[b] | $\ell$-CCO($^3\Sigma^-$)[b] |
|---|---|---|---|
| $F_{11}$ | 8.357 866 | 18.757 097 | 15.547 305 |
| $F_{21}$ | 0.365 540 | −0.206 468 | 1.119 727 |
| $F_{22}$ | 0.703 251 | 6.251 244 | 6.323 650 |
| $F_{33/44}$ | 8.563 429 | 0.264 816 | 0.291 883 |
| $F_{111}$ | −41.7268 | −125.5625 | −113.1874 |
| $F_{211}$ | −0.6029 | −0.0316 | −1.6699 |
| $F_{221}$ | −0.4480 | 0.1053 | −1.4711 |
| $F_{331/441}$ | −41.5576 | −0.7204 | −0.8905 |
| $F_{222}$ | −0.6955 | −35.7840 | −44.2481 |
| $F_{332/442}$ | 0.3912 | −0.1820 | −0.5236 |
| $F_{1111}$ | 181.89 | 679.57 | 669.36 |
| $F_{2111}$ | −0.47 | −0.05 | 1.79 |
| $F_{2211}$ | 0.30 | −0.95 | 0.57 |
| $F_{3311/4411}$ | 182.22 | 0.27 | 0.70 |
| $F_{2221}$ | 0.87 | −0.64 | 5.75 |
| $F_{3321/4421}$ | −1.23 | 0.35 | 1.80 |
| $F_{2222}$ | −0.81 | 185.04 | 212.77 |
| $F_{3322/4422}$ | −0.76 | 0.07 | −1.17 |
| $F_{3333/4444}$ | 183.44 | 0.89 | 2.29 |
| $F_{3344}$ | | 0.65 | 1.15 |
| $r_{e,1}$/pm | 95.755 605 | 115.257 717 | 115.751 957 |
| $r_{e,2}$/pm | 95.755 605 | 106.478 534 | 136.313 026 |
| $\angle_e$/° | 104.513 727 | 180.000 000 | 180.000 000 |

[a] Force constants in symmetry-internal displacement coordinates [Eq. (6) of the manuscript].

[b] Force constants in simple internal displacement coordinates [Eqs. (3)-(5) of the manuscript].

**go to summary**

Table S3: Vibrationally-averaged rotational constants (in MHz) for $c$-$H_2O(^1A_1)$, $\ell$-$HCN(^1\Sigma_g^+)$, and $\ell$-$CCO(^3\Sigma^-)$ model systems as obtained from our final QFFs (Table S2) and second-order perturbation theory (SPECTRO).

| | | Rotational constant | | | |
|---|---|---|---|---|---|
| Molecule | | QFF | Experiment[a] | \|Diff.\|[b] | % Error[c] |
| $c$-$H_2O(^1A_1)$ | $A_0$ | 832 984.7 | 835 755.4 | 2770.8 | 0.332 |
| | $B_0$ | 434 963.8 | 434 974.9 | 11.1 | 0.003 |
| | $C_0$ | 278 375.8 | 278 414.3 | 38.5 | 0.014 |
| $\ell$-$HCN(^1\Sigma_g^+)$ | $B_0$ | 44 352.4 | 44 316.0 | 36.5 | 0.082 |
| | $B_1$ | 44 035.5 | 44 003.5 | 32.0 | 0.073 |
| | $B_2$ | 44 450.9 | 44 422.4 | 28.4 | 0.064 |
| | $B_3$ | 44 051.6 | 44 013.8 | 37.8 | 0.086 |
| $\ell$-$CCO(^3\Sigma^-)$ | $B_0$ | 11 553.2 | 11 545.6 | 7.6 | 0.066 |
| | $B_1$ | 11 463.7 | 11 453.5 | 10.2 | 0.089 |
| | $B_2$ | 11 595.2 | 11 587.7 | 7.5 | 0.064 |
| | $B_3$ | 11 489.0 | 11 479.6 | 9.5 | 0.083 |
| Average[d] | | | | 271.8 | 0.087 |
| Average w/o $A_0$ $H_2O$[e] | | | | 21.9 | 0.062 |

[a] Refs. 1, 2, 3, 4.

[b] Absolute deviations between theory and experiment.

[c] Percent errors calculated using (|Diff.|/Experiment)×100%.

[d] Average quantities including all data.

[e] Average quantities without inclusion of water $A_0$.

**go to summary**

Table S4: Fundamental vibrational frequencies (in $cm^{-1}$) for $c$-$H_2O(^1A_1)$, $\ell$-$HCN(^1\Sigma_g^+)$, and $\ell$-$CCO(^3\Sigma^-)$ model systems as predicted from our final QFFs (Table S2) and second-order perturbation theory (SPECTRO).

| Molecule | | Vibrational band origin | | | |
|---|---|---|---|---|---|
| | | QFF | Experiment[a] | \|Diff.\|[b] | % Error[c] |
| $c$-$H_2O(^1A_1)$ | $\nu_1$ | 3653.7 | 3656.7 | 2.9 | 0.081 |
| | $\nu_2$ | 1595.9 | 1594.6 | 1.3 | 0.079 |
| | $\nu_3$ | 3751.9 | 3755.8 | 3.9 | 0.104 |
| $\ell$-$HCN(^1\Sigma_g^+)$ | $\nu_1$ | 3309.1 | 3311.5 | 2.4 | 0.072 |
| | $\nu_2$ | 714.8 | 713.5 | 1.4 | 0.193 |
| | $\nu_3$ | 2100.3 | 2096.8 | 3.4 | 0.163 |
| $\ell$-$CCO(^3\Sigma^-)$ | $\nu_1$ | 1978.9 | 1970.9 | 8.1 | 0.409 |
| | $\nu_2$ | 385.6 | 379.5 | 6.1 | 1.608 |
| | $\nu_3$ | 1066.2 | 1066.8 | 0.6 | 0.058 |
| Average[d] | | | | 3.3 | 0.307 |

[a] Refs. 1, 2, 3, 4.

[b] Absolute deviations between theory and experiment.

[c] Percent errors calculated using (|Diff.|/Experiment)×100%.

[d] Average quantities including all data.

**go to summary**

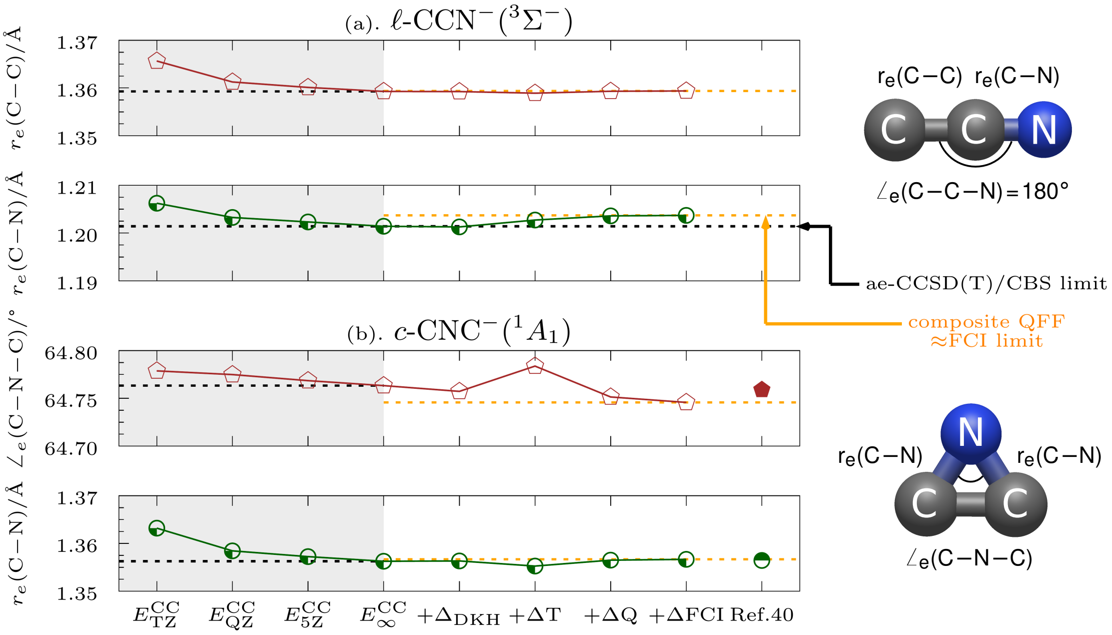


Figure S1: Convergence of the predicted equilibrium geometries for (a). $\ell$-$CCN^-(^3\Sigma^-)$ and (b). $c$-$CNC^-(^1A_1)$ as a function of each energy increment [see Eq. (7) of the paper]. For comparison, we also show the calculated values from the raw CC/ACV$XZ$ ($X = T, Q, 5$) QFFs separately as well as the most accurate results from the literature (Ref. 40 of the paper) for the $c$-$CNC^-$ species [panel (b)]. Shaded gray areas mark the transition region from one-particle to $\mathcal{N}$-particle expansion extrapolations. Black and orange lines highlight the corresponding geometries obtained at the one-particle CBS limit ($E_\infty^{CC}$) and from the final QFFs, respectively; ae stands for all electron (non-frozen-core) values.

**go to summary**

Table S5: Calculated nuclear spin-rotation interaction constants (**C** tensors) at the QFF equilibrium geometries for $\ell$-CCN$^-$($^3\Sigma^-$) and $c$-CNC$^-$($^1A_1$). Data obtained at the full-valence CASSCF/AV5Z level of theory using `DALTON`. Units are kHz.

| | $\ell$-CCN$^-$ | $\ell$-$^{13}$CCN$^-$ | $\ell$-C$^{13}$CN$^-$ | $\ell$-CC$^{15}$N$^-$ |
|---|---|---|---|---|
| $c_I(^{14}\mathrm{N})^a$ | 1.8802 | 1.8020(5.9405) | 1.8802(5.6409) | (2.5547) |
| | $c$-CNC$^-$ | $c$-$^{13}$CNC$^-$ | $c$-C$^{15}$NC$^-$ | |
| $C_{aa}(^{14}\mathrm{N})^a$ | 18.8880 | 18.5770(36.7986) | (−25.3831) | |
| $C_{bb}(^{14}\mathrm{N})^a$ | 14.3623 | 13.8507(36.9602) | (−20.1467) | |
| $C_{cc}(^{14}\mathrm{N})^a$ | −04762 | −0.4630(−0.4177) | (0.6543) | |

[a] Data evaluated at the $^{14}$N nucleus. The corresponding values obtained at $^{13}$C and $^{15}$N are given in parenthesis.

**go to summary**

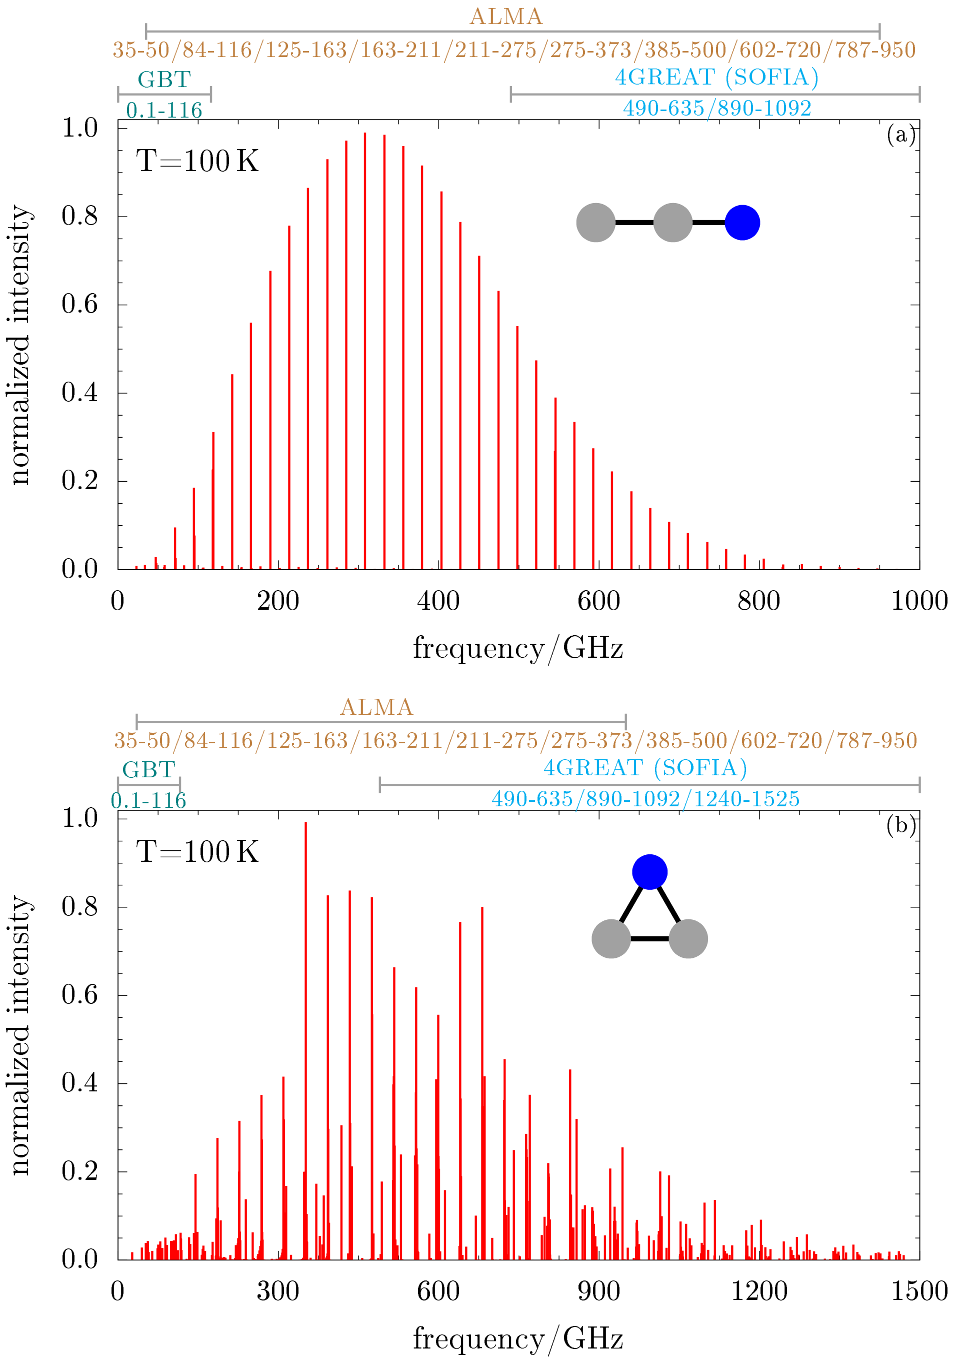


Figure S2: Simulated rotational spectra at $T = 100\,\mathrm{K}$ of (a). $\ell$-$CCN^-$($^3\Sigma^-$) and (b). $c$-$CNC^-$($^1A_1$) in their ground vibrational states. Working frequency ranges (in GHz) of the GBT, ALMA (from left to right: band 1, and bands 3 to 10) and the GREAT receiver bands (onboard the Stratospheric Observatory for Infrared Astronomy, SOFIA) are also displayed.

**go to summary**

```
<?xml version="1.0"?>
<Mixture Units="MHz" PrintLevel="plDefault" Version="PGOPHER 10.1.182
    04 Dec 2018 20:59  64 bit (fpc 3.3.1 x86_64-Linux)" PlotUnits="
   MHz">
  <Parameter Name="SmallE" Value="2E-18"/>
  <Species Name="Species" Jmax="100">
    <LinearMolecule Name="LinearMolecule" nNuclei="1" JAdjustSym="
        False">
      <LinearManifold Name="Ground" Initial="True" LimitSearch="True
          ">
        <Linear Name="v=0" S="2" Lambda="Sigma-">
          <Parameter Name="B" Value="11861.915"/>
          <Parameter Name="LambdaSS" Value="11958.871045849"/>
          <Parameter Name="gamma" Value="-19.16453035"/>
          <Parameter Name="D" Value="0.0061295907"/>
          <Parameter Name="H" Value="-2.4911113E-9"/>
          <LinearNucleus Name="Nucleus1" Spin="2">
            <Parameter Name="b" Value="25.2521"/>
            <Parameter Name="c" Value="-16.2363"/>
            <Parameter Name="eQq0" Value="-2.9088"/>
            <Parameter Name="cI" Value="0.0018802"/>
          </LinearNucleus>
        </Linear>
      </LinearManifold>
      <TransitionMoments Bra="Ground" Ket="Ground">
        <SphericalTransitionMoment Bra="v=0" Ket="v=0">
          <Parameter Name="Strength" Value="1.9873"/>
        </SphericalTransitionMoment>
      </TransitionMoments>
    </LinearMolecule>
  </Species>
  <Parameter Name="Temperature" Value="10"/>
  <Parameter Name="Fmin" Value="-6242.34857650319"/>
  <Parameter Name="Fmax" Value="300271.926137171"/>
  <FormSettings Name="ConstantsWindow" ActiveObject="LinearMolecule:
      Species - LinearMolecule"/>
</Mixture>
```


**go to summary**

```
<?xml version="1.0"?>
<Mixture Units="MHz" Version="PGOPHER 10.1.182 04 Dec 2018 20:59  64
    bit (fpc 3.3.1 x86_64-Linux)" PlotUnits="MHz">
  <Parameter Name="SmallE" Value="2E-18"/>
  <Species Name="Species" Jmax="60">
    <AsymmetricMolecule Name="AsymmetricTop" nNuclei="1" C2zAxis="b"
        PointGroup="C2v" eoWt="0" oeWt="0" JAdjustSym="False">
      <AsymmetricManifold Name="Ground" Initial="True">
        <AsymmetricTop Name="v=0">
          <Parameter Name="A" Value="43384.081"/>
          <Parameter Name="BBar" Value="30167.5775"/>
          <Parameter Name="BDelta" Value="19046.357"/>
          <Parameter Name="DK" Value="0.2062998257"/>
          <Parameter Name="DJK" Value="-0.0807246694"/>
          <Parameter Name="DJ" Value="0.1171867146"/>
          <Parameter Name="deltaK" Value="0.0867726315"/>
          <Parameter Name="deltaJ" Value="0.0494394954"/>
          <Parameter Name="HK" Value="0.0000198385516"/>
          <Parameter Name="HKJ" Value="-0.00002346133495"/>
          <Parameter Name="HJK" Value="5.884084373E-6"/>
          <Parameter Name="HJ" Value="9.114534222E-8"/>
          <Parameter Name="phiK" Value="-3.835427964E-7"/>
          <Parameter Name="phiJK" Value="2.239710312E-6"/>
          <Parameter Name="phiJ" Value="4.393211801E-8"/>
          <AsymmetricTopNucleus Name="Nucleus1" Spin="2">
            <Parameter Name="CHIzz" Value="5.0986"/>
            <Parameter Name="CHIxxmyy" Value="-2.5493"/>
            <Parameter Name="Caa" Value="0.018888002"/>
            <Parameter Name="Cbb" Value="0.014362263"/>
            <Parameter Name="Ccc" Value="-0.000476158"/>
          </AsymmetricTopNucleus>
        </AsymmetricTop>
      </AsymmetricManifold>
      <TransitionMoments Bra="Ground" Ket="Ground">
        <CartesianTransitionMoment Axis="b" Bra="v=0" Ket="v=0">
          <Parameter Name="Strength" Value="1.1011"/>
        </CartesianTransitionMoment>
      </TransitionMoments>
    </AsymmetricMolecule>
  </Species>
  <Parameter Name="Temperature" Value="10"/>
  <Parameter Name="Fmin" Value="-3040.22031910054"/>
  <Parameter Name="Fmax" Value="477889.273883812"/>
  <FormSettings Name="ConstantsWindow" ActiveObject="
      AsymmetricTopNucleus: Species - AsymmetricTop - Ground - v=0 -
      Nucleus1"/>
</Mixture>
```


## go to summary

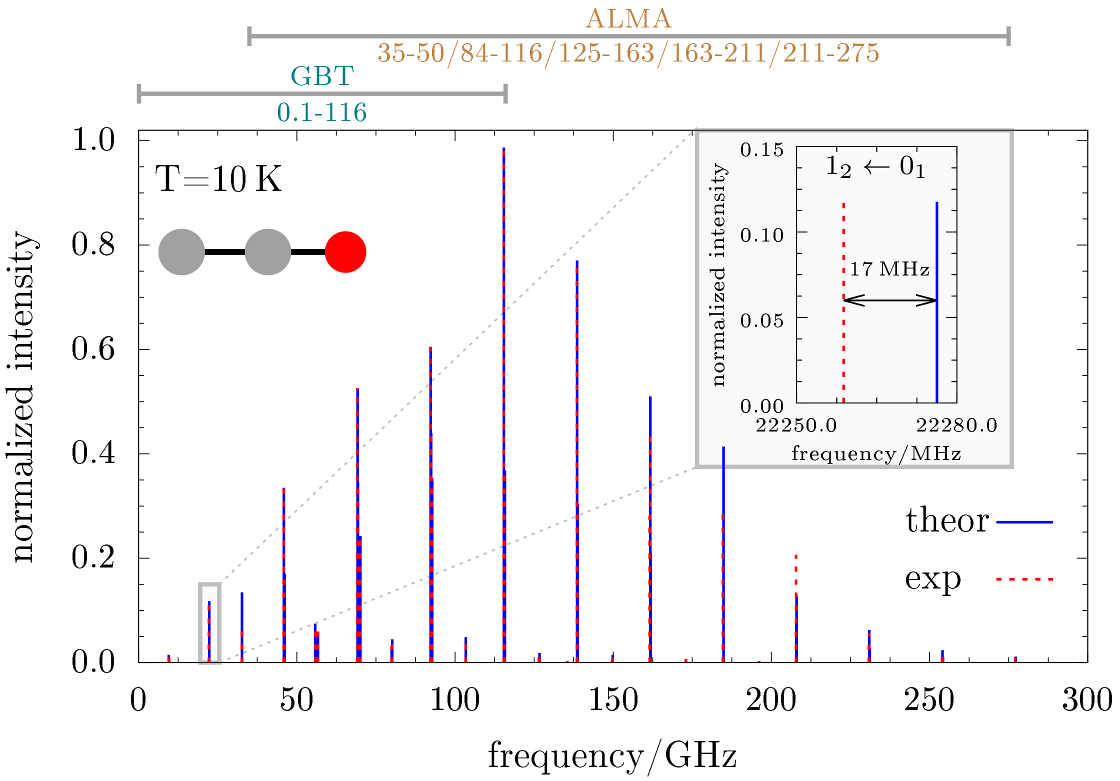


Figure S3: Simulated rotational spectra at 10 K of $\ell$-CCO($^3\Sigma^-$) in its ground vibrational state. The spectroscopic constants calculated in this work have been utilized in the theoretical simulation. They are: $B_0 = 11553.212$ MHz, $D = 0.005586297$ MHz, $H = -1.311221 \times 10^{-9}$ MHz, $\lambda = 11594.05$ MHz, and $\gamma = -15.04$ MHz. The correponding experimental values can be found in Ref. [3]. Working frequency ranges (in GHz) of the GBT and ALMA (from left to right: band 1, and bands 3 to 6) are also displayed.

**go to summary**

## References


[1] W. S. Benedict, N. Gailar, and E. K. Plyler, J. Chem. Phys. **24**, 1139 (1956).

[2] G. C. Mellau, B. P. Winnewisser, and M. Winnewisser, J. Mol. Spectrosc. **249**, 23 (2008).

[3] Z. Abusara, M. Dehghani, and N. Moazzen-Ahmadi, Chem. Phys. Lett. **417**, 206 (2006).

[4] N. Ohashi, R. Kiryu, S. Okino, and M. Fujitake, J. Mol. Spectrosc. **157**, 50 (1993).
